# Supplementary material for: Excitation energies from diffusion Monte Carlo using selected Configuration Interaction nodes
Source: arXiv:1805.09553 source file (2018-05-25)
Supplement: Supplementary file 1 [file ExQMC-SI.pdf]

# Supporting Information for "Excitations energies from diffusion Monte Carlo using selected Configuration Interaction nodes"

Anthony Scemama,[1] Anouar Benali,[2] Denis Jacquemin,[3] Michel Caffarel,[1] and Pierre-François Loos[1, a)]

[1)]*Laboratoire de Chimie et Physique Quantiques, Université de Toulouse, CNRS, UPS, France*

[2)]*Computational Science Division, Argonne National Laboratory, Argonne, IL 60439, United States of America*

[3)]*Laboratoire CEISAM - UMR CNRS 6230, Université de Nantes, 2 Rue de la Houssinière, BP 92208, 44322 Nantes Cedex 3, France*

## I. GEOMETRIES

Below are given the cartesian coordinates of the two compounds investigated in this study. These are provided in atomic units (bohr) and they have been obtained at the CC3(full)/AVTZ level of theory.

### A. Water

```
O    0.00000000         0.00000000        -0.13209669
H    0.00000000         1.43152878         0.97970006
H    0.00000000        -1.43152878         0.97970006
```

### B. Formaldehyde

```
C    0.00000000         0.00000000        -1.13947666
O    0.00000000         0.00000000         1.14402883
H    0.00000000         1.76627623        -2.23398653
H    0.00000000        -1.76627623        -2.23398653
```

[a)]Corresponding author: loos@irsamc.ups-tlse.fr

TABLE I. sCI and DMC total energies of the ground and various excited states of the water molecule obtained with the AVDZ, AVTZ and AVQZ Dunning's basis sets. The error bar corresponding to one standard error is reported in parenthesis.

| | Singlet states of $H_2O$ | | | | Triplet states of $H_2O$ | | |
|---|---|---|---|---|---|---|---|
| | $^1A_1$ | $^1B_1$ | $^1A_2$ | $^1A_1$ | $^3B_1$ | $^3A_2$ | $^3A_1$ |
| **sCI/AVDZ** | | | | | | | |
| sCI(4) | −76.224 611 | −75.935 727 | −75.858 219 | −75.840 734 | −75.966 237 | −75.888 464 | −75.873 243 |
| sCI(5) | −76.259 203 | −75.976 987 | −75.911 076 | −75.886 999 | −75.997 784 | −75.921 987 | −75.910 265 |
| sCI(6) | −76.269 278 | −75.991 236 | −75.925 495 | −75.902 522 | −76.006 609 | −75.932 100 | −75.920 012 |
| sCI(7) | −76.273 123 | −75.995 925 | −75.930 262 | −75.907 291 | −76.010 428 | −75.936 629 | −75.924 213 |
| exFCI | −76.274 528 | −75.997 706 | −75.932 093 | −75.909 184 | −76.011 979 | −75.938 424 | −75.925 877 |
| **sCI/AVTZ** | | | | | | | |
| sCI(4) | −76.253 328 | −75.961 011 | −75.884 794 | −75.867 528 | −75.997 294 | −75.914 224 | −75.906 152 |
| sCI(5) | −76.310 465 | −76.022 512 | −75.952 131 | −75.931 994 | −76.047 096 | −75.969 810 | −75.960 624 |
| sCI(6) | −76.330 401 | −76.048 162 | −75.982 106 | −75.960 098 | −76.065 195 | −75.990 163 | −75.980 019 |
| sCI(7) | −76.338 375 | −76.057 398 | −75.991 631 | −75.970 210 | −76.072 103 | −75.998 286 | −75.987 587 |
| exFCI | −76.342 770 | −76.062 535 | −75.997 095 | −75.975 760 | −76.076 339 | −76.003 196 | −75.992 155 |
| **sCI/AVQZ** | | | | | | | |
| sCI(4) | −76.251 182 | −75.963 458 | −75.895 400 | −75.871 394 | −76.003 028 | −75.921 446 | −75.912 553 |
| sCI(5) | −76.310 735 | −76.021 940 | −75.953 862 | −75.933 645 | −76.056 641 | −75.979 375 | −75.969 484 |
| sCI(6) | −76.336 815 | −76.053 302 | −75.986 672 | −75.965 831 | −76.078 582 | −76.003 328 | −75.993 549 |
| sCI(7) | −76.348 678 | −76.065 456 | −75.999 645 | −75.978 241 | −76.087 511 | −76.013 704 | −76.003 205 |
| exFCI | −76.362 851 | −76.080 586 | −76.015 279 | −75.994 396 | −76.095 197 | −76.022 118 | −76.011 320 |
| **DMC/AVDZ** | | | | | | | |
| sCI(4) | −76.4211(2) | −76.1382(2) | −76.0719(1) | −76.0497(2) | −76.1525(1) | −76.0805(1) | −76.0685(1) |
| sCI(5) | −76.4240(2) | −76.1401(2) | −76.0756(1) | −76.0532(2) | −76.1548(1) | −76.0821(1) | −76.0710(1) |
| sCI(6) | −76.4261(3) | −76.1419(3) | −76.0773(3) | −76.0550(3) | −76.1561(1) | −76.0834(2) | −76.0724(2) |
| sCI(7) | −76.4261(7) | −76.1436(6) | −76.0795(7) | −76.0552(7) | −76.1561(2) | −76.0842(6) | −76.0730(6) |
| exFCI | −76.4270(4) | −76.1431(4) | −76.0785(4) | −76.0557(4) | −76.1567(1) | −76.0843(3) | −76.0733(3) |
| **DMC/AVTZ** | | | | | | | |
| sCI(4) | −76.4247(1) | −76.1422(1) | −76.0760(1) | −76.0540(1) | −76.1562(1) | −76.0838(1) | −76.0728(1) |
| sCI(5) | −76.4301(2) | −76.1463(2) | −76.0806(2) | −76.0590(2) | −76.1608(2) | −76.0876(1) | −76.0774(1) |
| sCI(6) | −76.4316(4) | −76.1490(4) | −76.0827(4) | −76.0619(5) | −76.1630(2) | −76.0896(2) | −76.0794(2) |
| sCI(7) | −76.4341(5) | −76.1507(5) | −76.0865(5) | −76.0641(5) | −76.1632(3) | −76.0910(3) | −76.0811(3) |
| exFCI | −76.4339(5) | −76.1510(4) | −76.0858(4) | −76.0644(4) | −76.1639(2) | −76.0912(2) | −76.0812(2) |
| **DMC/AVQZ** | | | | | | | |
| sCI(4) | −76.4255(1) | −76.1427(1) | −76.0770(1) | −76.0552(1) | −76.1572(1) | −76.0846(1) | −76.0733(1) |
| sCI(5) | −76.4308(2) | −76.1463(2) | −76.0813(2) | −76.0596(2) | −76.1623(1) | −76.0888(1) | −76.0787(1) |
| sCI(6) | −76.4326(2) | −76.1492(2) | −76.0845(2) | −76.0632(2) | −76.1646(2) | −76.0914(2) | −76.0804(2) |
| sCI(7) | −76.4339(2) | −76.1500(2) | −76.0853(2) | −76.0644(2) | −76.1658(3) | −76.0927(3) | −76.0822(3) |
| exFCI | −76.4348(3) | −76.1515(3) | −76.0869(3) | −76.0663(3) | −76.1665(3) | −76.0936(3) | −76.0825(3) |

TABLE II. sCI and DMC extrapolated total energies of the ground and various excited states of the water molecule obtained with the AVDZ, AVTZ and AVQZ Dunning's basis sets. The complete basis set (CBS) values are also reported. The error bar corresponding to one standard error is reported in parenthesis.

| State | exFCI energies | | | | exDMC energies | | | |
|---|---|---|---|---|---|---|---|---|
| | AVDZ | AVTZ | AVQZ | CBS | AVDZ | AVTZ | AVQZ | CBS |
| $^1A_1$ | −76.274 528 | −76.342 770 | −76.362 851 | −76.381 391 | −76.4270(4) | −76.4339(5) | −76.4348(3) | −76.4366(3) |
| $^1B_1$ | −75.997 706 | −76.062 535 | −76.080 586 | −76.098 407 | −76.1431(4) | −76.1510(4) | −76.1515(3) | −76.1536(3) |
| $^1A_2$ | −75.932 093 | −75.997 095 | −76.015 279 | −76.033 131 | −76.0785(4) | −76.0858(4) | −76.0869(3) | −76.0889(3) |
| $^1A_1$ | −75.909 184 | −75.975 760 | −75.994 396 | −76.012 677 | −76.0557(4) | −76.0644(4) | −76.0663(3) | −76.0686(3) |
| $^3B_1$ | −76.011 979 | −76.076 339 | −76.095 197 | −76.112 699 | −76.1567(1) | −76.1639(2) | −76.1665(3) | −76.1683(2) |
| $^3A_2$ | −75.938 424 | −76.003 196 | −76.022 118 | −76.039 744 | −76.0843(3) | −76.0912(2) | −76.0936(3) | −76.0954(3) |
| $^3A_1$ | −75.925 877 | −75.992 155 | −76.011 320 | −76.029 395 | −76.0733(3) | −76.0812(2) | −76.0825(3) | −76.085(3) |

TABLE III. sCI and DMC total energies of the ground and various excited states of the formaldehyde molecule obtained with the AVDZ Dunning's basis set. The extrapolated sCI and DMC energies, labeled as exFCI and exDMC respectively, are also reported. The error bar corresponding to one standard error is reported in parenthesis.

| | Singlet states of $CH_2O$ | | | | | | Triplet states of $CH_2O$ | | | | |
|---|---|---|---|---|---|---|---|---|---|---|---|
| | $^1A_1$ | $^1A_2$ | $^1B_2$ | $^1B_2$ | $^1A_1$ | $^1A_2$ | $^3A_2$ | $^3A_1$ | $^3B_2$ | $^3B_2$ | $^3A_1$ |
| **sCI/AVDZ** | | | | | | | | | | | |
| sCI(4) | −114.110 867 | −113.897 394 | −113.779 339 | −113.740 752 | −113.741 452 | −113.668 992 | −113.991 630 | −113.868 233 | −113.821 573 | −113.785 142 | −113.782 432 |
| sCI(5) | −114.191 389 | −114.014 626 | −113.888 886 | −113.852 080 | −113.851 576 | −113.785 170 | −114.061 333 | −113.959 182 | −113.917 436 | −113.881 687 | −113.878 339 |
| sCI(6) | −114.216 042 | −114.058 864 | −113.939 252 | −113.903 193 | −113.902 546 | −113.862 993 | −114.087 412 | −113.994 302 | −113.958 082 | −113.923 555 | −113.919 216 |
| exFCI | −114.245 851 | −114.099 251 | −113.984 602 | −113.950 401 | −113.947 574 | −113.927 812 | −114.114 376 | −114.021 911 | −113.990 552 | −113.957 002 | −113.951 717 |
| **DMC/AVDZ** | | | | | | | | | | | |
| sCI(4) | −114.4828(3) | −114.3287(3) | −114.2083(3) | −114.1755(3) | −114.1723(3) | −114.1543(5) | −114.3502(3) | −114.2569(3) | −114.2144(3) | −114.1823(3) | −114.1768(3) |
| sCI(5) | −114.4865(5) | −114.3370(7) | −114.2152(5) | −114.1820(5) | −114.1810(6) | −114.1592(6) | −114.3529(3) | −114.2616(4) | −114.2213(4) | −114.1889(4) | −114.1833(4) |
| sCI(6) | −114.4882(7) | −114.3385(7) | −114.2184(7) | −114.1848(7) | −114.1822(7) | −114.1685(7) | −114.3549(7) | −114.2633(8) | −114.2237(7) | −114.1910(7) | −114.1858(6) |
| exDMC | −114.4893(6) | −114.3417(7) | −114.2212(7) | −114.1876(7) | −114.1864(7) | −114.1710(9) | −114.3553(5) | −114.2647(6) | −114.2263(6) | −114.1936(6) | −114.1881(6) |

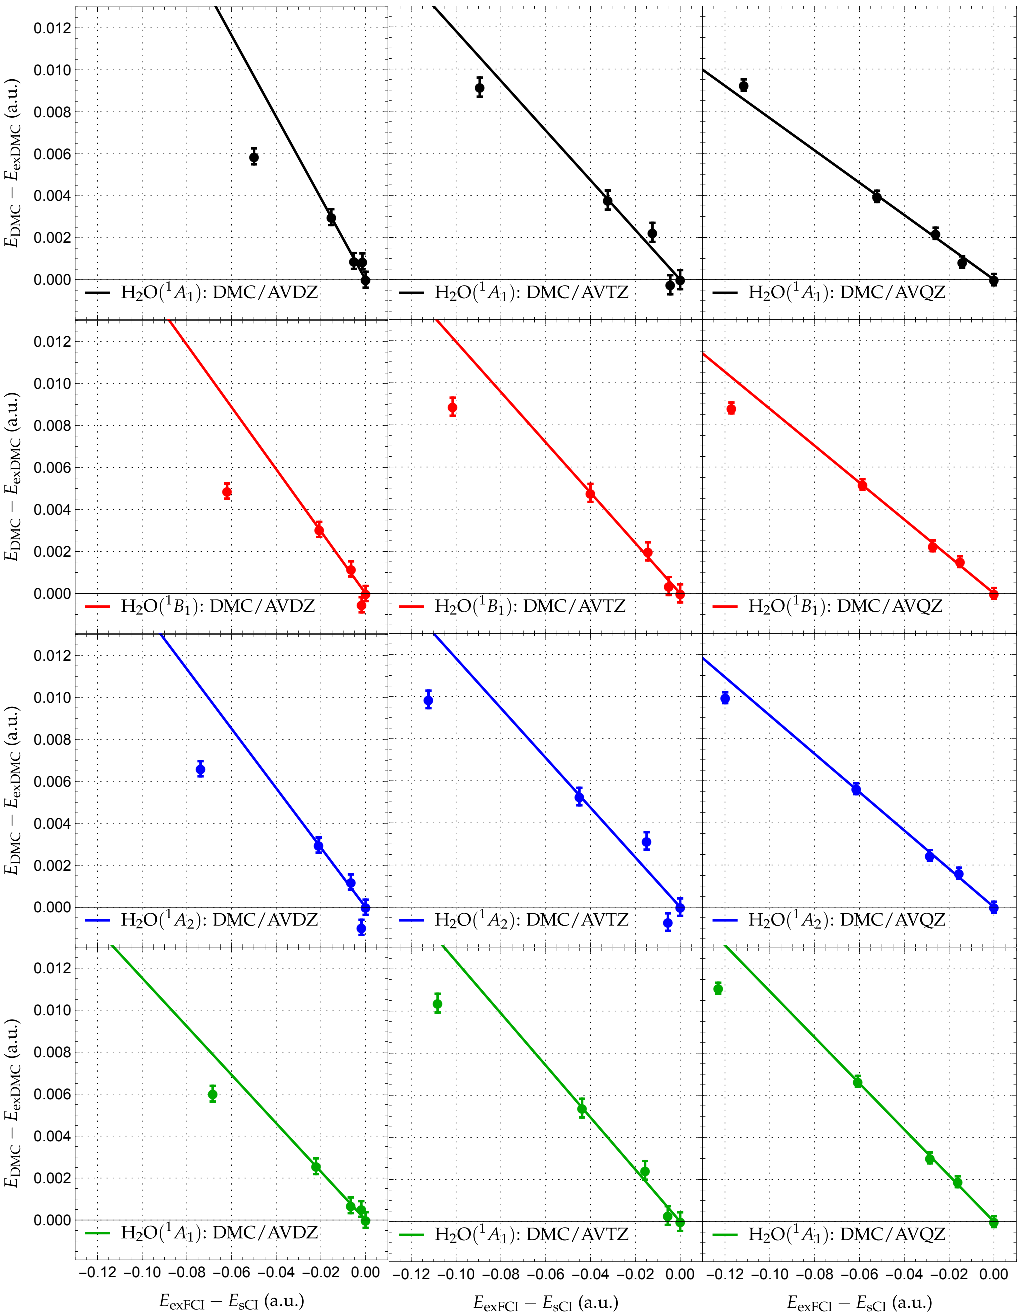


FIG. 1. Extrapolation of the DMC energies for the singlet ground and excited states of the water molecule with the AVDZ, AVTZ and AVQZ Dunning's basis sets. $E_{sCI}$ is the variational sCI energy, while $E_{exFCI}$ and $E_{exDMC}$ are the extrapolated sCI and DMC energies, respectively. The last three points are taken into account in the linear extrapolation.

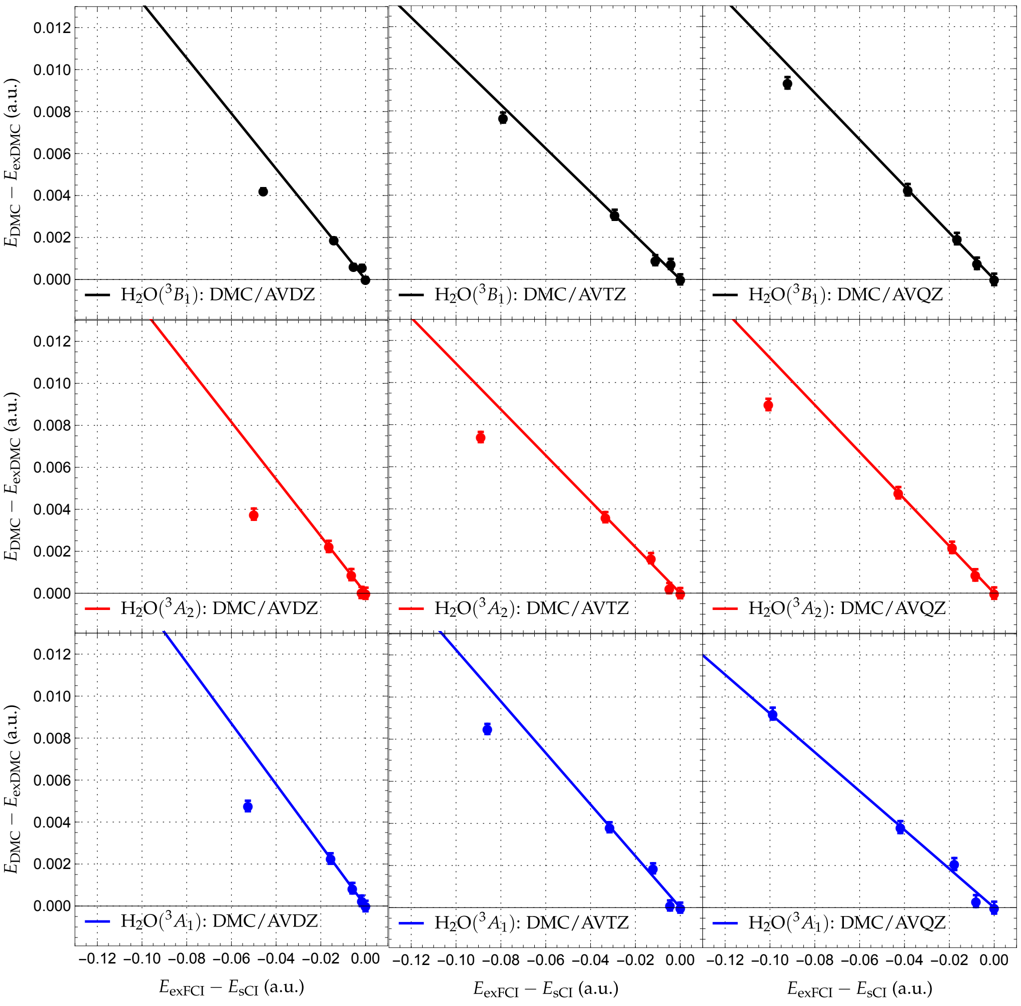


FIG. 2. Extrapolation of the DMC energies for the triplet excited states of the water molecule with the AVDZ, AVTZ and AVQZ Dunning's basis sets. $E_{\text{sCI}}$ is the variational sCI energy, $E_{\text{DMC}}$ is the DMC energy, while $E_{\text{exFCI}}$ and $E_{\text{exDMC}}$ are the extrapolated sCI and DMC energies, respectively. The last three points are taken into account in the linear extrapolation.

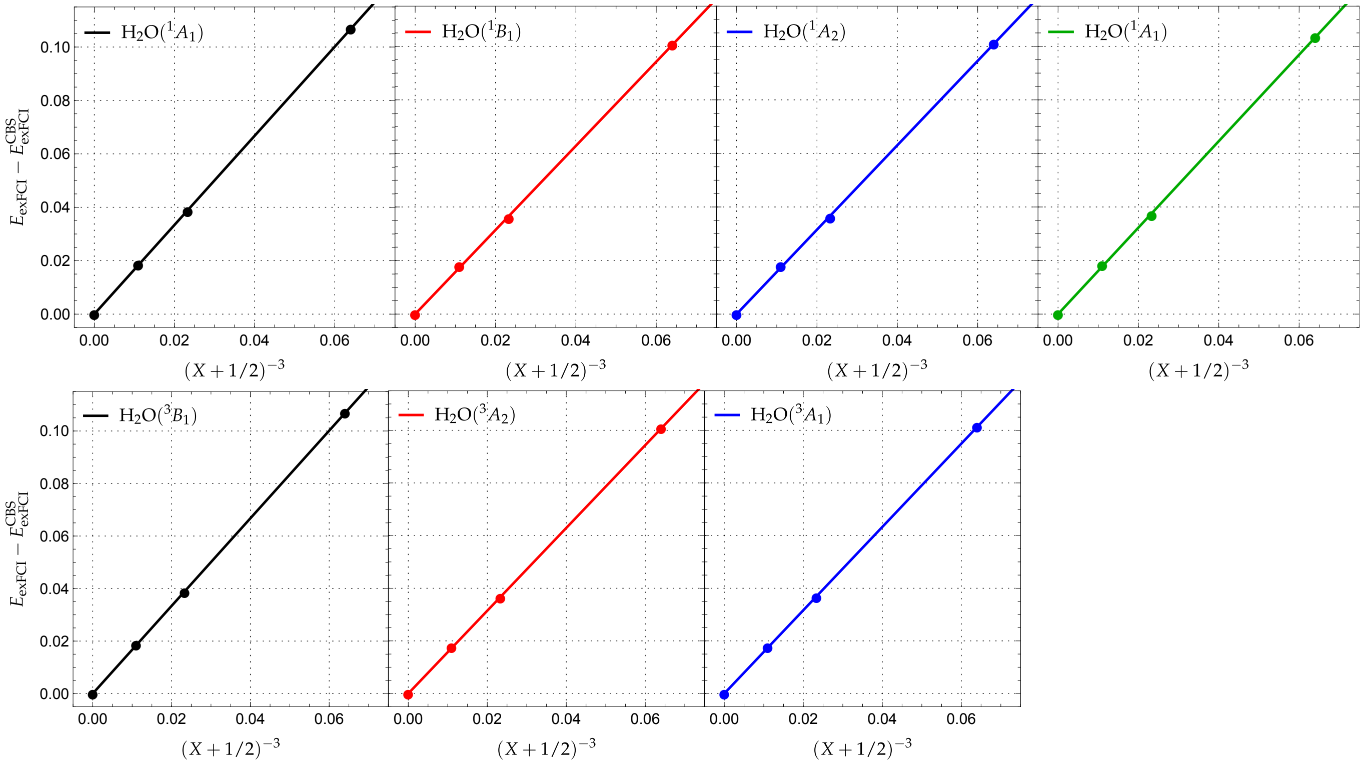


FIG. 3. Extrapolation of the exFCI energies to the complete basis set (CBS) limit for the water molecule. The extrapolated sCI energy $E_{exFCI}$ is plotted as a function of $(X + 1/2)^{-3}$ for $X = 2$ (AVDZ), $X = 3$ (AVTZ) and $X = 4$ (AVQZ). $E_{exFCI}^{CBS}$ stands for the CBS energy obtained at the exFCI level.

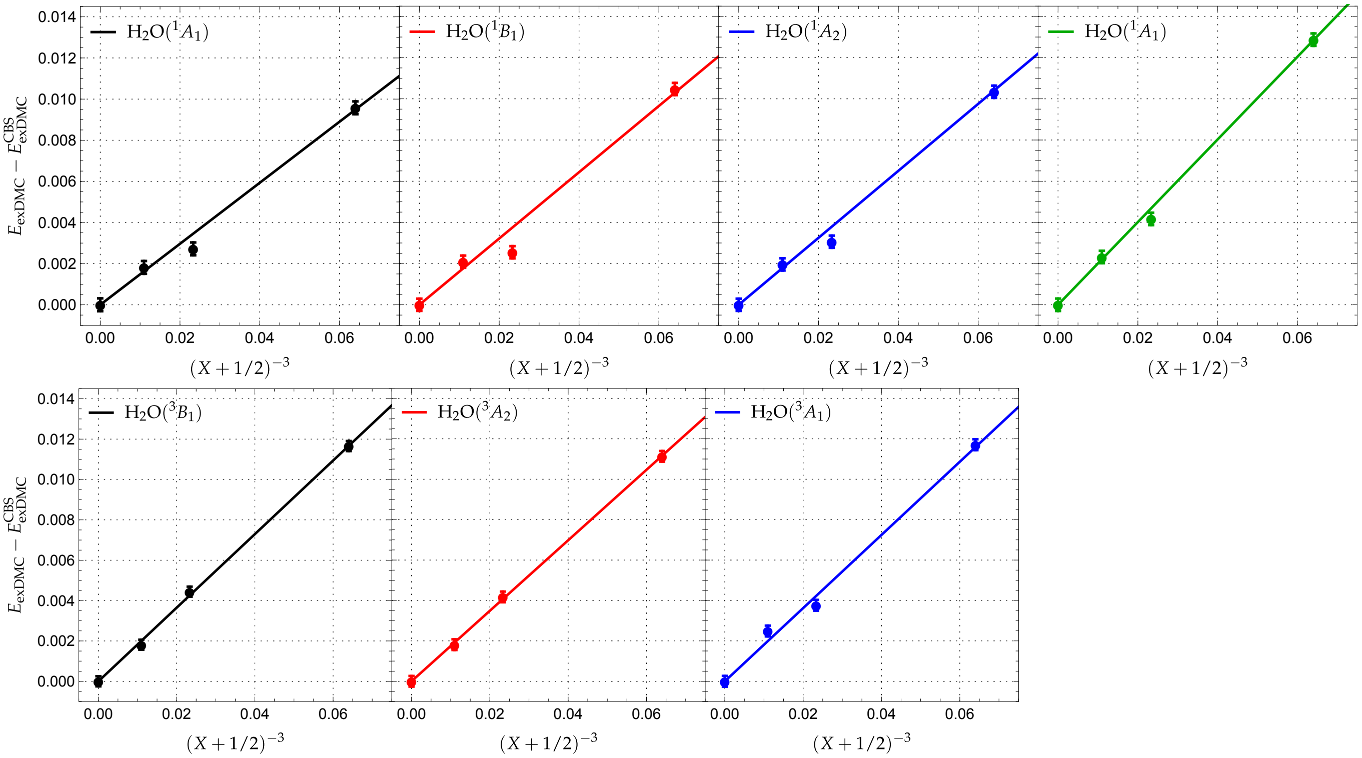


FIG. 4. Extrapolation of the exDMC energies to the complete basis set (CBS) limit for the water molecule. The extrapolated DMC energy $E_{\text{exDMC}}$ is plotted as a function of $(X+1/2)^{-3}$ for $X = 2$ (AVDZ), $X = 3$ (AVTZ) and $X = 4$ (AVQZ). $E_{\text{exDMC}}^{\text{CBS}}$ stands for the CBS energy obtained at the exDMC level.

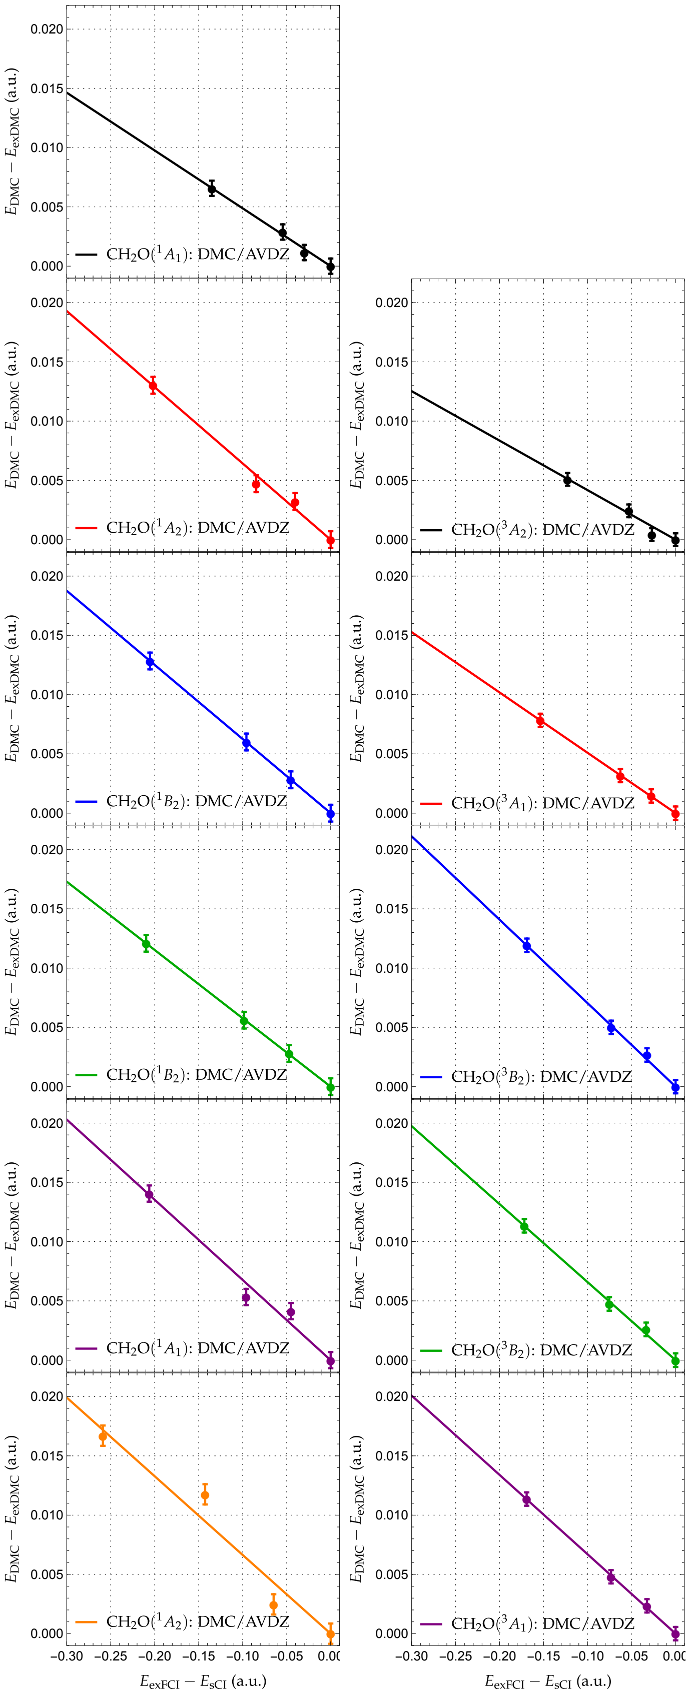


FIG. 5. Extrapolation of the DMC energies for the singlet ground and excited states (left) and the triplet excited states (right) of the water molecule with the AVDZ and AVTZ Dunning's basis sets. $E_{sCI}$ is the variational sCI energy, $E_{DMC}$ is the DMC energy, while $E_{exFCI}$ and $E_{exDMC}$ are the extrapolated sCI and DMC energies, respectively. All the points are taken into account in the linear extrapolation.
